# Supplementary material for: TransGNN: Harnessing the Collaborative Power of Transformers and Graph Neural Networks for Recommender Systems
Source: arXiv:2308.14355 source file (2024-05-18)
Supplement: Supplementary file 1 [file appendix.tex]

\section{Notes on the Experimental Setup}
\subsection{Details of Datasets}
\label{sec:data}

\par We evaluate the proposed model on five real-world representative datasets (\textit{i.e.,} Yelp, Gowalla, Tmall, Amazon-Book, and MovieLens), which vary significantly in domains and sparsity:
\begin{itemize}
    \item \textbf{Yelp}: This commonly-used dataset contains user ratings on business venues collected from Yelp. Following other papers on implicit feedback~\cite{huang2021knowledge}, we treat users’ rated venues as interacted items and treat unrated venues as non-interacted items.
    \item \textbf{Gowalla}: It contains users’ check-in records on geographical locations obtained from Gowalla. This evaluation dataset is generated from the period between 2016 and 2019.
    \item \textbf{Tmall}: This E-commerce dataset is released by Tmall, containing users’ behaviors for online shopping. We collect the page-view interactions during December in 2017.
    \item \textbf{Amazon-Book}: Amazon-review is a widely used dataset for
product recommendation~\cite{he2016ups}. We select Amazon-book from the
collection. Similarly, we use the 10-core setting to ensure that each
user and item have at least ten interactions.
    \item \textbf{MovieLens}: This is a popular benchmark dataset for
evaluating recommendation algorithms~\cite{harper2015movielens}. In this work, we adopt the well-established version, MovieLens 10m (\textbf{ML-10m}), which contains about 10 million ratings of 10681 movies by 71567 users. The users of MovieLens 10M dataset are randomly chosen and each user rated at least 20 movies.
\end{itemize}

For dataset preprocessing, we follow the common practice in~\cite{huang2021knowledge,xia2022self,tang2018personalized}. For all datasets, we convert all numeric ratings or the presence of a review to implicit feedback of 1 (\textit{i.e.,} the user interacted with the item). After that, we group the interaction records by users and build the interaction sequence for each user by sorting these interaction records according to the timestamps. To ensure the quality of the dataset, following the common practice~\cite{huang2021knowledge,xia2022self,tang2018personalized,sun2019bert4rec}, we filtered out users and items with too few interactions. 

\subsection{Evaluation Protocols.} 
Following the recent collaborative filtering models~\cite{he2020lightgcn,wu2021self}, we adopt all-rank evaluation protocol. Under this protocol, during the evaluation of a user, both the positive items from the test set and all the non-interacted items are collectively ranked and assessed. For the assessment of recommendation performance, we have opted for widely recognized metrics, namely, \textbf{Recall@N} and Normalized Discounted Cumulative Gain (\textbf{NDCG@N})~\cite{ren2020sequential,wang2019neural}. The value of N in these metrics is set to 20 and 40.

\subsection{Details of Baselines}
\label{sec:baseline}

We evaluate our TransGNN by comparing it with 12 baselines from different research lines for comprehensive evaluation:

\noindent \textbf{Autoencoder-based Collaborative Filtering Approach.}
\begin{itemize}
    \item \textbf{AutoR}~\cite{sedhain2015autorec}: This model improves user/item representations with a three-layer autoencoder trained under a behavior reconstruction task.
\end{itemize}

\noindent \textbf{Graph Neural Networks for Recommendation.}
\begin{itemize}
    \item \textbf{GCMC}~\cite{berg2017graph}: This is one of the pioneering work to apply graph convolutional networks (GCNs) to the matrix completion task.
    \item \textbf{PinSage}~\cite{ying2018graph}:It applies random sampling in graph convolutional framework to study the collaborative filtering task.
    \item \textbf{NGCF}~\cite{wang2019neural}: This graph convolution-based approach additionally takes source-target representation interaction learning into consideration when designing its graph encoder.
    % \item \textbf{STGCN}~\cite{zhang2019star}: The model combines conventional graph convolutional encoders with graph autoencoders to improve the model robustness against sparse and cold-start samples.
    \item \textbf{LightGCN}~\cite{he2020lightgcn}: This work conducts in-depth analysis to study the effectiveness of modules in standard GCN for collaborative data, and proposes a simplified GCN model for recommendation.
    \item \textbf{GCCF}~\cite{chen2020revisiting}: This is another method which simplifies the GCNs by removing the non-linear transformation. In GCCF, the effectiveness of residual connections across graph iterations is validated.
\end{itemize}

% \noindent \textbf{Disentangled Graph Model for Recommendation.}
% \begin{itemize}
%     \item \textbf{DGCF}~\cite{wang2020disentangled}: It disentangles user interactions into multiple latent intentions to model user preference in a fine-grained way.
% \end{itemize}

\noindent \textbf{Hypergraph-based Neural Collaborative Filtering.}
\begin{itemize}
    \item \textbf{HyRec}~\cite{wang2020next}: This is a sequential collaborative model that learns item-wise high-order relations with hypergraphs.
    \item \textbf{DHCF}~\cite{ji2020dual}: This model adopts dual-channel hypergraph neural networks for both users and items in collaborative filtering.
\end{itemize}

\noindent \textbf{Recommenders enhanced by Self-Supervised Learning.} 
\begin{itemize}
    \item \textbf{MHCN}~\cite{yu2021self}: This model maximizes the mutual information between node embeddings and global readout representations, to regularize the representation learning for interaction graph.
    \item \textbf{SLRec}~\cite{yao2021self}: This approach employs the contrastive learning between the node features as regularization terms to enhance the existing recommender systems.
    \item \textbf{SGL}~\cite{wu2021self}: This model conducts data augmentation through random walk and feature dropout to generate multiple views. It enhances LightGCN with self-supervised contrastive learning.
\end{itemize}

\noindent \textbf{Recommenders enhanced by Hypergraph Transformer and Self-Supervised Learning}
\begin{itemize}
    \item \textbf{SHT}~\cite{xia2022self}: This model adopts a Self-Supervised Hypergraph Transformer framework (SHT) which augments user representations by exploring the global collaborative relationships in an explicit way.
\end{itemize}
